# Supplementary material for: Predicting Quality of Video Gaming Experience Using Global-Scale Telemetry Data and Federated Learning
Source: arXiv:2412.08950 source file (2025-02-26)
Supplement: Supplementary file 1 [file appendix.tex]

\section{Description of features in the dataset}

In this appendix, we provide the name and description for player and game features used in the data analysis and deep learning model:

\begin{table*}[]
\centering
\caption{Attributes and Descriptions of Game Data}
\begin{tabular}{|l|l|}
\hline
\textbf{Attribute} & \textbf{Description} \\ \hline
ID & A unique identifier for each game. \\ \hline
Category & Type of game, e.g., Main Game, DLC/Add-on, Expansion. \\ \hline
First Release Date & Initial release date. \\ & Impacts optimization for modern hardware. \\ \hline
Platforms & Platforms available, focus on PC. \\ \hline
Genres & Game genres like Action, Adventure, impacting FPS. \\ \hline
Game Modes & Available modes like Single-player, Multiplayer. \\ \hline
Player Perspectives & Game play perspective, e.g., First person, Third person. \\ \hline
Themes & Overarching themes, e.g., Fantasy, Science fiction. \\ \hline
Language Supports & Languages supported by the game. \\ \hline
Age Ratings & Age suitability ratings. \\ \hline
Follows & Number of followers or interest garnered. \\ \hline
Aggregated Rating & Average rating by critics. \\ \hline
Aggregated Rating Count & Number of aggregated ratings. \\ \hline
Rating & Average user rating. \\ \hline
Rating Count & Number of user ratings. \\ \hline
Total Rating & Overall rating combining user and critic ratings. \\ \hline
Total Rating Count & Total number of ratings. \\ \hline
DLCs & Downloadable content available. \\ \hline
Game Localizations & Game's availability in different regions. \\ \hline
\end{tabular}\label{tab:gamefeat}
\label{tab:game_data}
\end{table*}

% \begin{table*}[]
% \centering
% \caption{Attributes and Descriptions of Session Data}
% \begin{tabular}{|l|l|}
% \hline
% \textbf{Attribute} & \textbf{Description} \\ \hline
% Guid & Unique identifier of the player. \\ \hline
% Start Time & The hour, day, weekday, month, and year components of the local time timestamp \\ & when the executable came into foreground. \\ \hline
% Duration & Total time the application is in the foreground in the current session. \\ \hline
% Proc Name & Name of the foreground application (e.g., excel.exe). \\ \hline
% Longest Windowed Mode & Longest mode of a display device, Window mode or Full mode. \\ \hline
% Longest Non Responsive & Indicates if the session had non-responsive periods \\ & (True if `\textasciitilde' is present in process name). \\ \hline
% Longest Mode & Game/Non-Game Mode. \\ \hline
% Session Max Val & Max 5-sec FPS sample in the current session. \\ \hline
% Fps Bin & Count of 5-second FPS intervals recorded during the session. \\ \hline
% Session Avg Fps & Average FPS per session in the corresponding mode. \\ \hline
% Session Std Dev & Standard deviation of all 5-sec FPS sample bins. \\ \hline
% Last Session Start Time & Timestamp when exe came into foreground (local time) \\ & for the last session of the same player. \\ \hline
% Delta Time From Last Session & The time between the last session and this session \\ & of the same player. \\ \hline
% \end{tabular}
% \label{tab:session_data}
% \end{table*}

\begin{table*}[]
\centering
\caption{Attributes and Descriptions of Player Data}
\begin{tabular}{|l|l|}
\hline
\textbf{Attribute} & \textbf{Description} \\ \hline
Guid & Unique identifier of the client. \\ \hline
% Start Time & The hour and weekday components of the timestamp for the player's first game session. \\ \hline
% End Time & The hour and weekday components of the timestamp for the player's last game session. \\ \hline
Avg Session Per Month & The average amount of game sessions initiated by the player per month. \\ \hline
Avg Duration Per Session & the average duration of game sessions initiated by the player. \\ \hline
Game Portion & The percentage of the total duration of game sessions relative to all sessions combined. \\ \hline
Distinct Game Count & The count of distinct games the player played. \\ \hline
% Top1 Game Duration Pcnt & The percentage of the total duration attributed to the game \\ & with the longest duration compared to all games the player played. \\ \hline
% Top3 Game Duration Pcnt & The percentage of the total duration attributed to the top three games \\ & with the longest durations compared to all games the player played. \\ \hline
Windowed Mode & Mode of a display device, Window mode or Full mode. Default is Unknown. \\ \hline
Mode & Whether Game/non-Game mode is used more during the gaming processes. \\ \hline
Country Name & Location where the device is used (This is captured based on where the data is uploaded from). \\ \hline
% Persona & A user classification based on the types of applications used. \\ \hline
Device Age Category & A computed estimated measure based on the CPU launch date and the System First Boot Date. \\ \hline
Chassis Type & Device Form Factor - Notebook, Desktop, Server, etc. \\ \hline
Model Vendor & Device Manufacturer / OEM. \\ \hline
OS & Operating System. \\ \hline
RAM & Device RAM Size (Unit: GB). \\ \hline
CPU Process Node & CPU Process Node (unit: nm). \\ \hline
CPU Processor Number & The Number of CPU Processor Cores. \\ \hline
CPU Vendor & CPU Manufacturer. \\ \hline
Graphics Card Class & Graphics Card Category (This information is captured from publicly available metadata). \\ \hline
Discrete Graphics & Flag indicating if the system has an integrated or discrete graphics card. \\ \hline
Graphics Manuf & Graphics Manufacturer. \\ \hline
Vpro Enabled & Flag indicating if the system is vpro enabled. \\ \hline
Report Lifecycle Day & Life cycle of report(in days) = datediff(day, firstreportdate, lastreportdate). \\ \hline
Screensize Category & Device display size \\ & (For notebooks, it is the laptop screen size; for other form factors, it is the most used display size). \\ \hline
Window Desktop Portion & The percentage of the game window size relative to the desktop size. \\ \hline
\end{tabular}
\label{tab:player_data}
\end{table*}
